# Supplementary material for: Enhancing Descriptive Captions with Visual Attributes for Multimodal Perception
Source: arXiv:2412.14233 source file (2026-01-27)
Supplement: Supplementary file 1 [file main_appendix.tex]

% CVPR 2026 Paper Template; see https://github.com/cvpr-org/author-kit

\documentclass[10pt,twocolumn,letterpaper]{article}

%%%%%%%%% PAPER TYPE  - PLEASE UPDATE FOR FINAL VERSION
% \usepackage{cvpr}              % To produce the CAMERA-READY version
\usepackage[review]{cvpr}      % To produce the REVIEW version
\usepackage{graphicx}
\usepackage{booktabs}
\usepackage{colortbl}
\usepackage{makecell}
\usepackage{tikz,pgfplots,pgfplotstable}
\usepackage{color}
\usepackage{amsfonts}
\usepackage{amssymb}
\usepackage{arydshln}
\usepackage{multirow}
\usepackage{tcolorbox}

% Import additional packages in the preamble file, before hyperref
\input{preamble}

% It is strongly recommended to use hyperref, especially for the review version.
% hyperref with option pagebackref eases the reviewers' job.
% Please disable hyperref *only* if you encounter grave issues, 
% e.g. with the file validation for the camera-ready version.
%
% If you comment hyperref and then uncomment it, you should delete *.aux before re-running LaTeX.
% (Or just hit 'q' on the first LaTeX run, let it finish, and you should be clear).
\definecolor{cvprblue}{rgb}{0.21,0.49,0.74}
\definecolor{object_skyblue}{rgb}{0.405, 0.794, 0.902}
\definecolor{aquamarine}{rgb}{0.4, 1.0, 0.6}
\definecolor{ocr_coral}{rgb}{0.749,0.565,0}
\definecolor{hoi_green}{rgb}{0.492,0.671,0.333}
\usepackage[pagebackref,breaklinks,colorlinks,allcolors=cvprblue]{hyperref}

%%%%%%%%% PAPER ID  - PLEASE UPDATE
 % *** Enter the Paper ID here

%%%%%%%%% TITLE - PLEASE UPDATE
\title{Enhancing Descriptive Captions with Visual Attributes for Multimodal Perception -- Supplementary Material}

%%%%%%%%% AUTHORS - PLEASE UPDATE
\author{First Author\\
Institution1\\
Institution1 address\\
{\tt\small firstauthor@i1.org}
% For a paper whose authors are all at the same institution,
% omit the following lines up until the closing ``}''.
% Additional authors and addresses can be added with ``\and'',
% just like the second author.
% To save space, use either the email address or home page, not both
\and
Second Author\\
Institution2\\
First line of institution2 address\\
{\tt\small secondauthor@i2.org}
}

\begin{document}
\maketitle
% \input{sec/0_abstract}    
% \input{sec/1_intro}
% \input{sec/2_related}
% \input{sec/3_methods}
% \input{sec/4_experiments}
% \input{sec/5_conclusion}

% \clearpage
\input{sec/Appendix}
% WARNING: do not forget to delete the supplementary pages from your submission 
% \input{sec/X_suppl}
{
    \small
    \bibliographystyle{ieeenat_fullname}
    \bibliography{main}
}
\end{document}
